# Supplementary material for: Random lasing in an Anderson localizing optical fiber
Source: arXiv:1612.03835 source file (2017-06-02)
Supplement: Supplementary file 1 [file Supplementary.pdf]

# Random lasing in an Anderson localizing optical fiber

Behnam Abaie[1,2], Esmaeil Mobini[1,2], Salman Karbasi[3], Thomas Hawkins[4], John Ballato[4], and Arash Mafi[1,2*]

[1] *Department of Physics & Astronomy, University of New Mexico, Albuquerque, NM 87131, USA.*

[2] *Center for High Technology Materials, University of New Mexico, Albuquerque, NM 87106, USA.*

[3] *Department of Electrical and Computer Engineering, University of California, San Diego, La Jolla, CA 92093, USA.*

[4] *Center for Optical Materials Science and Engineering Technologies (COMSET) and the Department of Materials Science and Engineering, Clemson University, Clemson, SC 29634, USA.* [*] *Corresponding author: mafi@unm.edu*

## 1. Beam quality of g-ALOF laser output

Here we present the experimental results regarding the beam quality evaluation of the directional g-ALOF random laser. The $\sigma$ method [1,2] is applied. The experimental setup is presented in Fig. S1a. The output of g-ALOF laser is captured by a microscope objective and a CCD beam profiler is used to record the pattern. The pattern is recorded at its minimum beam width and a few other neighboring distances and is fitted to a quadratic function of $Z$ (distance from the focal point) from which the value of $M^2$ is extracted. The output pattern at two distances from the focal point are shown in Fig. S1b, and c. An $M^2 \approx 16$ is achieved for a typical lasing mode using this approach, which is of the order of $M^2$ values reported for higher order modes of a multimode step-index fiber.

We also point out that directionality of the random laser presented in this work is due to the guided nature of g-ALOF. The approximate numerical aperture of the fiber which is calculated from the index difference of the high-index ($n_1$) and low-index spots ($n_2$) determines the sine of the far-field emission angle where for $\Delta n = 0.1$, the cone is approximately 30-degrees which is highly directional. Also note that because of the guided nature of the fiber-based random laser, collecting the laser light with a high-NA microscope objective is substantially more efficient in this work.

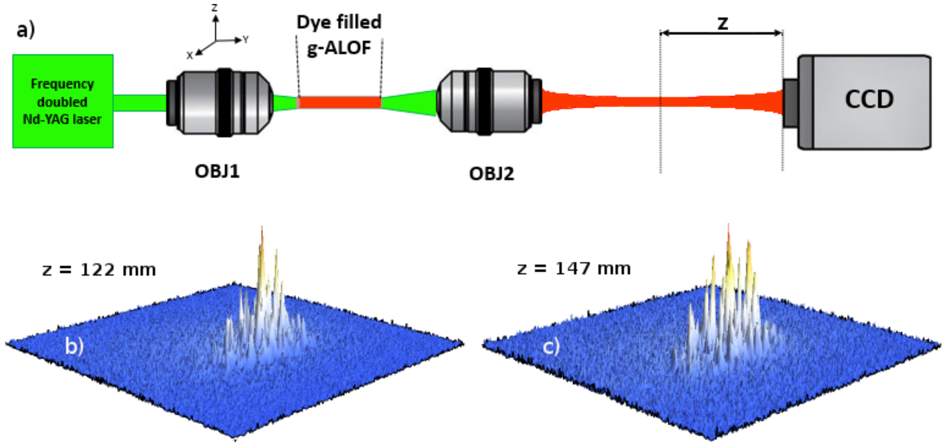


Figure S 1 – $M^2$ **measurement of g-ALOF laser.** a) The experimental setup; the output of g-ALOF laser is captured by a microscope objective and a CCD beam profiler is used to record the pattern. The recorded patterns at z = 122, and 147 mm are presented in b, and c, respectively.

## 2. Dependency of the spectral stability to localization strength

To further investigate the impact of localization strength on the spectral stability of the laser, here we present a comparison between the laser emission spectra in two different levels of localization strength; dye solutions with two different values of refractive index are used and the spectral stability of two lasing modes in g-ALOF filled with these solutions are compared. For a higher refractive index contrast in the Fig. S2a, a strongly localized mode is excited in the system and a high spectral stability is observed ($NMISE \approx 3\%$). However, by reducing the refractive index contrast in Fig. S2b ($\Delta n = 0.06$), modes become less localized and spatially broader. The recorded laser spectra in this case is significantly broader along with chaotic fluctuations. The value of $NMISE$ calculated for the less localized lasing mode is around 12% indicative of the higher level of fluctuations in the emission spectra.

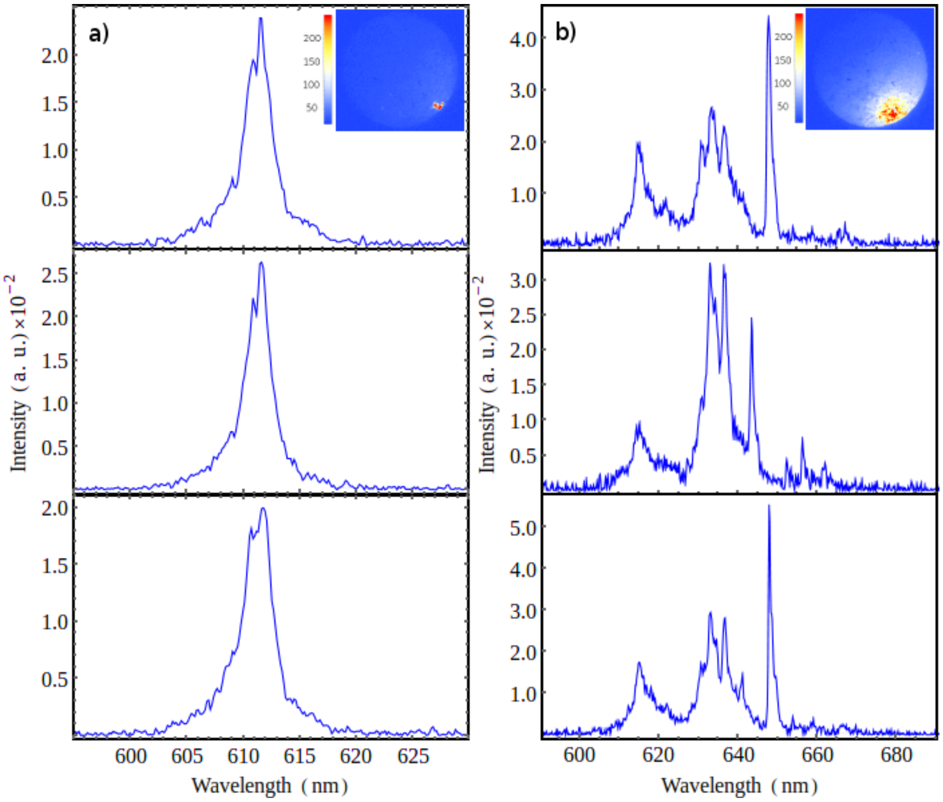


Figure S 2 – **Dependency of the spectral stability to the localization strength.** a) A large refractive index contrast between the g-ALOF host glass and the dye solution is used. The lasing mode is strongly localized and the emission spectra is highly stable ($NMISE \approx 3\%$). b) a lower refractive index contrast in the disordered system, reduces the localization strength. The lasing mode is less localized and spatially broader. The emission spectra shows a higher level of fluctuations ($NMISE \approx 12\%$).

## 3. Spatial coherency of g-ALOF laser

Here we present the experimental results regarding spatial coherence of the g-ALOF laser source. The output of the random laser in the Anderson localized regime ($NMISE \approx 3\%$), under extended input pumping, is used to perform Young double slit experiment [3, 4]. The experimental setup and the interference pattern achieved by random laser illumination is shown in Fig. S3. In this figure, part a is the experimental setup where the output is collected by OBJ2 and used to illuminate the double slit of width 80 µm and center-

to-center spacing 500 µm. The interference pattern is reordered by a CCD beam profiler. Part b shows the pattern formed when the double slit is illuminated by the output of g-ALOF laser, and part c shows the intensity distribution along a narrow horizontal line crossing the interference pattern in part b. Part d and e are interference pattern and intensity distribution when the double slit experiment is repeated with a spatially coherent He-Ne laser. For the random laser case, no interference pattern is observed, verifying spatial incoherence of the random laser. From a physical point of view, several localized lasing modes randomly distributed across the transverse dimension of g-ALOF with random phase lase and beat incoherently.

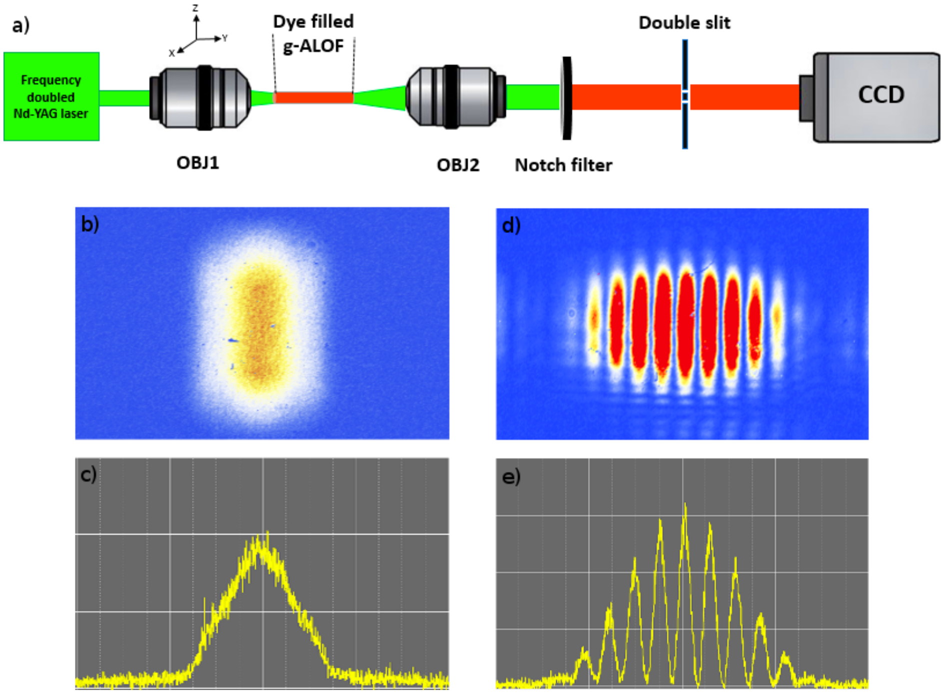


Figure S 3 – **Coherency measurement of g-ALOF laser.** a) Experimental setup; the g-ALOF laser output is collected by OBJ2 and used to illuminate the double slit of width 80 µm and center-to-center spacing 500 µm. b) The interference pattern formed when the double slit is illuminated by the output of g-ALOF laser, and c) the intensity distribution along a narrow horizontal line crossing the interference pattern in part b. d) and e) are interference pattern and intensity distribution when the double slit experiment is repeated with a He-Ne laser.

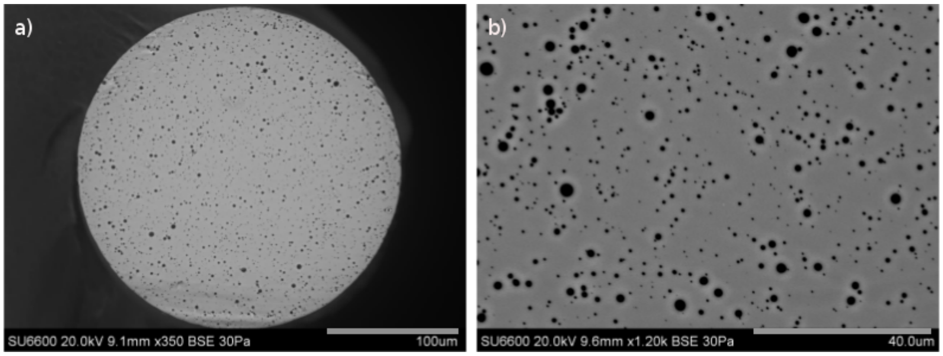


Figure S 4 – **Scanning electron microscope (SEM) image of g-ALOF.** a) SEM image of the tip of g-ALOF. The darker sites are the airholes. b) Magnified SEM image shows the details of the air-holes in a portion of the fiber cross section.

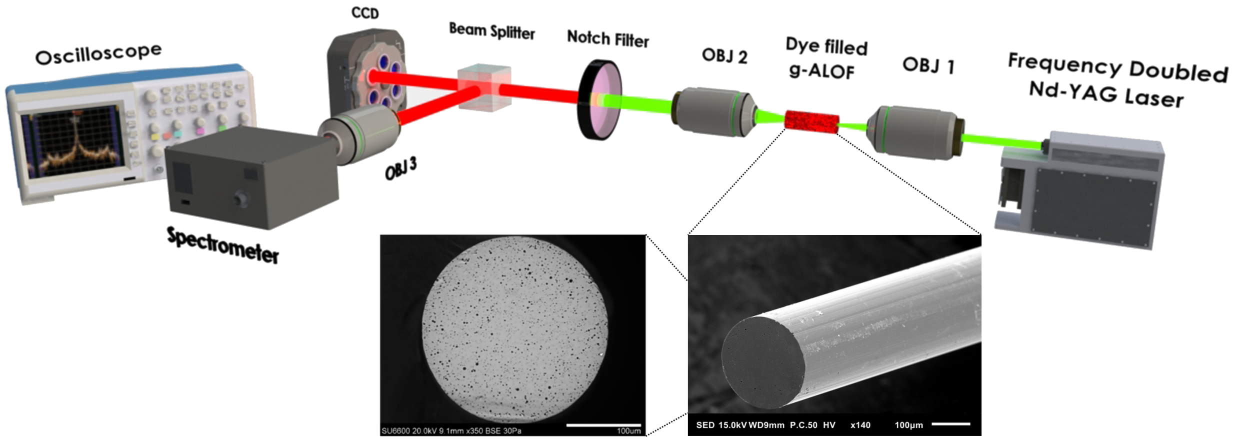


Figure S 5 – **Experimental setup.** The dye-filled g-ALOF is end-pumped using a frequency-doubled Nd:YAG laser with a pulse duration of 0.6ns. A microscope objective (OBJ1) is implemented on an XYZ translation stage to scan the focused pump beam across g-ALOF input facet. The black and white SEM image shows the details of the tip of g-ALOF (the darker sites are the air-holes randomly paced across the transverse structure of the fiber). Near-field image of the tip of g-ALOF at the output facet is captured by another objective (OBJ2) and recorded by a CCD beam profiler. The pump (or laser) is filtered by a notch filter. A beam splitter (BS) is used to direct laser beam towards a spectrometer or a fast oscilloscope for spectrum and time analysis.

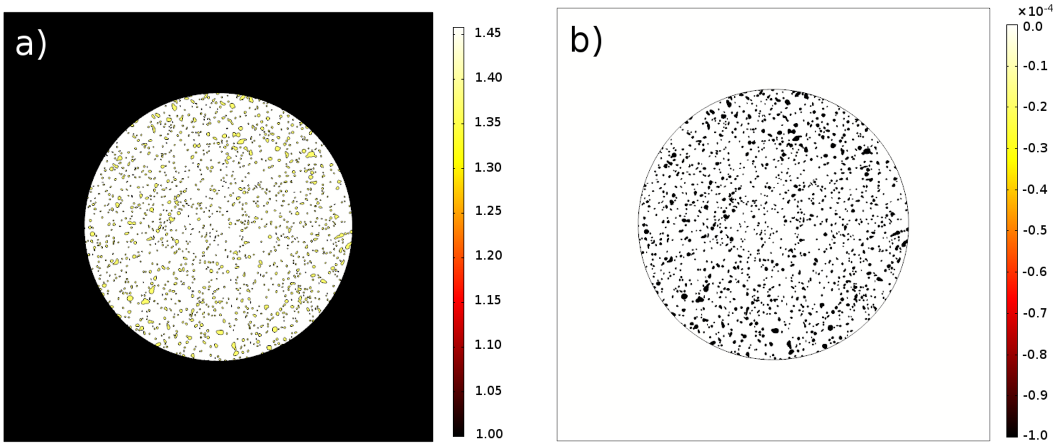


Figure S 6 – **Refractive index profile used in the simulations.** a) real part, and b) imaginary part of the refractive index. The pattern is directly extracted from the SEM image of g-ALOF.

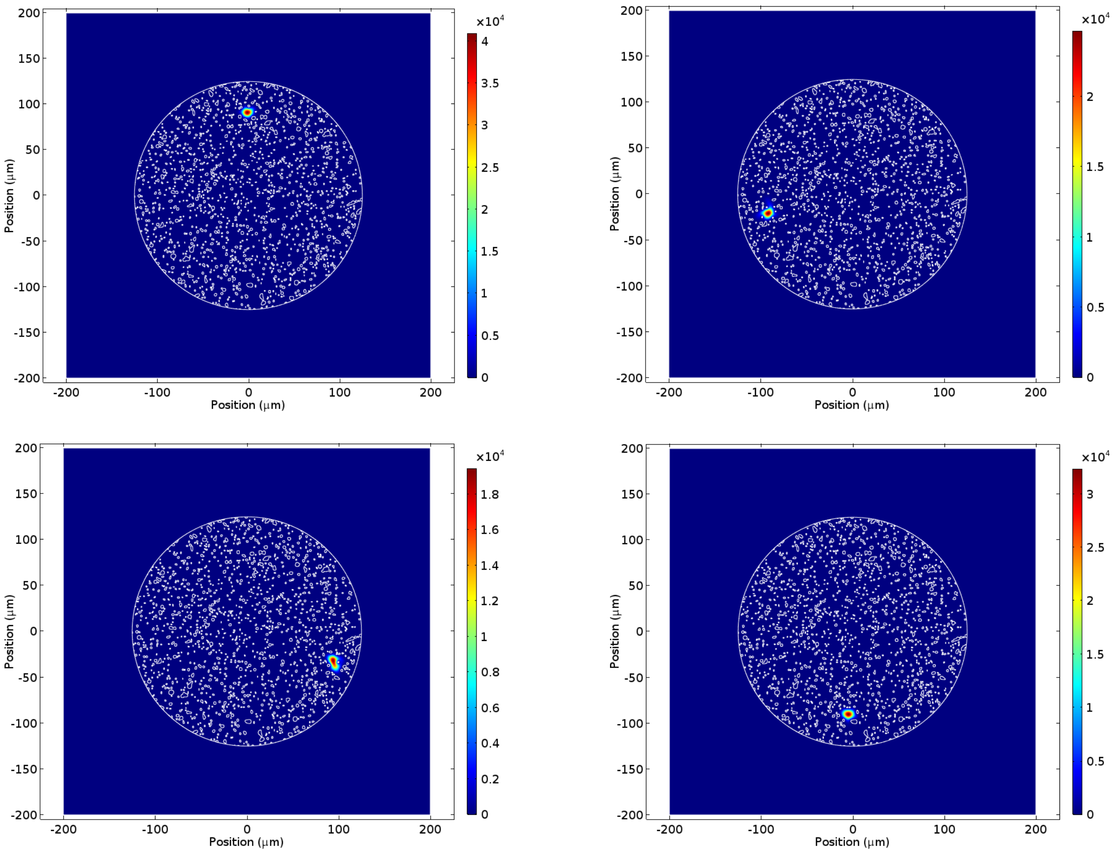


Figure S 7 – **More examples of calculated localized modes.** The localized modes are mainly located near the edges of g-ALOF where disorder is stronger.

## References


1. Siegman, A. How to (maybe) measure laser beam quality (1998).
2. Mafi, A. & Moloney, J. V. Beam quality of photonic-crystal fibers. *Journal of lightwave technology* **23**, 2267–2270 (2005).
3. Redding, B., Choma, M. A. & Cao, H. Spatial coherence of random laser emission. *Optics letters* **36**, 3404–3406 (2011).
4. Hokr, B. H. *et al.* A narrow-band speckle-free light source via random raman lasing. *Journal of Modern Optics* **63**, 46–49 (2016).
